# Supplementary material for: Kernel-Based Tests for Likelihood-Free Hypothesis Testing
Source: arXiv:2308.09043 source file (2023-11-23)
Supplement: Supplementary file 1 [file supplement.tex]

\documentclass{article}
% if you need to pass options to natbib, use, e.g.:
%     \PassOptionsToPackage{numbers, compress}{natbib}
% before loading neurips_2023
% ready for submission
\usepackage[nonatbib,final]{neurips_2023}
% to compile a preprint version, e.g., for submission to arXiv, add add the
% [preprint] option:
%     \usepackage[preprint]{neurips_2023}
% to compile a camera-ready version, add the [final] option, e.g.:
%     \usepackage[final]{neurips_2023}
% to avoid loading the natbib package, add option nonatbib:
% \usepackage[nonatbib]{neurips_2023}
\usepackage[utf8]{inputenc} % allow utf-8 input
\usepackage[T1]{fontenc}    % use 8-bit T1 fonts
\usepackage{hyperref}       % hyperlinks
\usepackage{url}            % simple URL typesetting
\usepackage{booktabs}       % professional-quality tables
\usepackage{amsfonts}       % blackboard math symbols
\usepackage{nicefrac}       % compact symbols for 1/2, etc.
\usepackage{microtype}      % microtypography
\usepackage{xcolor}         % colors
\hypersetup{
    colorlinks,
    linkcolor={blue!50!black},
    citecolor={blue!50!black},
    urlcolor={blue!80!black}
}
\usepackage{wrapfig}
\usepackage{amsmath}
\usepackage{amssymb}
\usepackage{mathtools}
\usepackage{amsthm}
\usepackage{bbm}
\usepackage{braket}
\usepackage{minitoc}
\usepackage[capitalize,noabbrev]{cleveref}
\usepackage{algorithm} 
\usepackage{algorithmic}

\usepackage[sort]{natbib}
\setcitestyle{numbers,open={[},close={]}}
\bibliographystyle{abbrvnat_Neurips_ours}
% \bibliographystyle{abbrvnat}
% \bibliographystyle{plain}
% \rui{I don't find full name of some of the ref authors, use abbrvnat. removed URLs}
%\bibliographystyle{icml2023}

%%%%% Theorem %%%%%
\theoremstyle{plain}

\theoremstyle{definition}

\theoremstyle{remark}

%%%%% New commands %%%%%
\input{commands}

\usepackage{xr}
\makeatletter
\newcommand*{\addFileDependency}[1]{
  \typeout{(#1)}
  \@addtofilelist{#1}
  \IfFileExists{#1}{}{\typeout{No file #1.}}
}
\makeatother

\newcommand*{\myexternaldocument}[1]{
    \externaldocument{#1}
    \addFileDependency{#1.tex}
    \addFileDependency{#1.aux}
}

\myexternaldocument{Neurips/submission}

\title{Supplement to ``Kernel-based tests for Likelihood-Free Hypothesis Testing''}
%\DeclareMathOperator*{\argmin}{arg\,min}

% The \author macro works with any number of authors. There are two commands
% used to separate the names and addresses of multiple authors: \And and \AND.
%
% Using \And between authors leaves it to LaTeX to determine where to break the
% lines. Using \AND forces a line break at that point. So, if LaTeX puts 3 of 4
% authors names on the first line, and the last on the second line, try using
% \AND instead of \And before the third author name.

\author{%
  Patrik R\'obert Gerber\thanks{Equal contribution.} \\
  Department of Mathematics, MIT \\
  Cambridge, MA 02139 \\
  \texttt{prgerber@mit.edu} 
  \\
  \And Tianze Jiang\footnotemark[1]  \\ Department of Mathematics, MIT \\
  Cambridge, MA 02139 \\
  \texttt{tjiang@mit.edu} 
  \\
  \And Yury Polyanskiy\footnotemark[1]  \\ Department of EECS, MIT \\ Cambridge, MA 02139 \\ \texttt{yp@mit.edu} 
  \\ 
  \And Rui Sun\footnotemark[1]  \\ Department of Mathematics, MIT \\ Cambridge, MA 02139 \\ \texttt{eruisun@mit.edu}
}

\setcounter{algorithm}{1}
\setcounter{figure}{3}

\begin{document}

\maketitle

\tableofcontents
\appendix
\onecolumn

\input{appendix}

\bibliography{bib}

\end{document}
